# Supplementary material for: Trust Under Siege: Label Spoofing Attacks against Machine Learning for Android Malware Detection
Source: arXiv:2503.11841 source file (2026-08-31)
Supplement: Supplementary file 1 [file appendix.tex]

\appendix
\section{Appendix}

\subsection{Experiment Results}
\label{apx:exp_results}
Here we report results of Deep KNN against both availability and integrity attacks for Drebin and MaMaDroid features.
